# Supplementary material for: Window Token Concatenation for Efficient Visual Large Language Models
Source: arXiv:2504.04024 source file (2025-04-05)
Supplement: Supplementary file 1 [file appendix.tex]

\appendix

\section{Broader impact discussion}

Since our WiCo ($+$) serves as one of the components of current VLLMs, it still faces the same potential issues. We provide all the possible risks and possible mitigation strategies as follows:

\textbf{Safety and security risks}. VLLMs can be misused to create convincing phishing content or to automate the production of harmful or malicious media. To solve these problems, we can implement strict use-case restrictions and user authentication protocols. Also, regularly updating and auditing models to detect and mitigate emergent misuse patterns is important.

\textbf{Discrimination and biases}. VLLMs might amplify existing societal biases present in training data, leading to discriminatory outputs against certain groups. We can use de-biasing techniques during training and engage in continuous monitoring and adjustment post-deployment.

\textbf{Deceptions}. VLLMs can generate hyper-realistic content could lead to the creation of deepfakes or misleading information that can deceive the public. To guard public property security, we can develop digital watermarking and content provenance tools to verify authenticity. It is necessary to educate users and deploy fact-checking tools alongside model outputs.

\textbf{Privacy concerns}. VLLMs could unintentionally memorize and regurgitate private or sensitive information included in the training data. We can implement differential privacy during training, use federated learning where feasible, and conduct privacy audits to ensure data protection.

\textbf{Human rights implications}. Misuse of VLLMs in surveillance applications or content moderation could impinge on freedom of expression and information. We can establish clear ethical guidelines and usage policies emphasizing human rights. 

\textbf{Environmental impact}. Although our method can help with efficient training, large-scale training still requires substantial computational resources, contributing to carbon emissions. 

Despite these potential risks, we believe our method will be beneficial for both the research community and the whole society. 
Through diligent application of the mitigation strategies outlined, we can enhance the safety and effectiveness of our technology, making it an efficient tool for building and deploying the general AI assistant. 

\section{More visualization results}
We provide more visualization results of the frozen features and tuned ones in \cref{fig:more_vis_results}. From the visualization, we can observe that the tuned CLIP features are smoother than the frozen ones. The smoothness in the features maps is beneficial for combining the local information.
\begin{figure}
    \centering
    \includegraphics[width=1\linewidth]{figures/feature_vis1.pdf}
    \caption{The visual feature map (mean pooling) comparison of frozen features and tuned ones. The frozen features are extracted by the frozen CLIP, and the tuned features are learned by tuning the last few layers of the CLIP.}
    \label{fig:more_vis_results}
\end{figure}

\section{Licenses for existing assets}

All the assets used in our paper have been publicly released, which are given as follows:

\begin{enumerate}
    \item \textbf{LLaVA-1.5}: codes: \url{https://github.com/haotian-liu/LLaVA}, datasets: \url{https://huggingface.co/datasets/liuhaotian/LLaVA-Instruct-150K}, under Apache-2.0 license;
    \item \textbf{Shikra}:
    codes: \url{https://github.com/shikras/shikra}, under Creative Commons Corporation license;
    \item \textbf{VQAv2}: \url{https://visualqa.org/download.html};
    \item \textbf{ScienceQA}: \url{https://scienceqa.github.io/};
    \item \textbf{TextVQA}: \url{https://textvqa.org/};
    \item \textbf{POPE}: \url{https://github.com/RUCAIBox/POPE};
    \item \textbf{MME}: \url{https://github.com/BradyFU/Awesome-Multimodal-Large-Language-Models};
    \item \textbf{MMBench}: \url{https://github.com/open-compass/MMBench};
    \item \textbf{RefCOCO, RefCOCO+, RefCOCOg}: \url{https://github.com/lichengunc/refer}
    
\end{enumerate}

\section*{Ethical statement}
All the datasets and models utilized in our paper are  public available. These models and datasets are widely used in vision language model research community. 
% Additionally, the original documentation of these assets ensures compliance with the ethical guidelines, like the absence of privacy or offensive content.

We acknowledge that the improper use of VLLMs can lead to biases, as well as privacy or security concerns. It is crucial for future research and commercial applications to address these issues and ensure their fair and responsible deployment. The findings and techniques presented in this paper comply with applicable licenses and align with their intended use.
